# Supplementary material for: Pattern formation of spherical particles in an oscillating flow
Source: arXiv:2305.01564 source file (2023-05-02)
Supplement: Supplementary file 1 [file Appendix.tex]

% We study the role of particle-bottom friction on the streamwise motion of a single particle in an oscillating box filled with viscous fluid, using the numerical code by \citet{breugem2012second}. This code is also used to uncover the physical mechanism behind the chain interactions, as described in Sec.~\ref{sec:mechanism}.
% In this section, a single spherical particle is placed inside a double periodic box with lateral dimensions of $20\times10$ and a height of 5 diameters. The flow is solved on a uniform Cartesian grid with a grid spacing of $D/24$ and the particles are simulated using an immersed boundary method.
% We further set $A/D=0.909$, $\delta/D\approx0.0265$, $\Gamma=0.75$, and $s=7.5$, i.e. closely matching the experimental conditions for which $A_r/D=0.5$.
% The value of the Coulomb friction coefficient $\mu_c$ is varied between $0.0$ and $0.5$.

% Figure~\ref{fig:velocity_muc} shows, for three different values of $\mu_c$, the velocities as a function of time during the 20th oscillation period, when the system has reached a quasi-steady state and the transients have died out. The velocities are normalized by the velocity amplitude of the box, $2\pi A f$, and time is normalized by the oscillation frequency, $f$, such that one unit of time corresponds to one oscillation period.

% In the absence of particle-bottom friction ($\mu_c=0.0$, in Fig.~\ref{fig:velocity_muc}(a)), the particle rotation, represented by the dash-dotted curve, is approximately zero. The hydrodynamic interactions cause slight rotation of the particle, but these effects are sufficiently small to be insignificant for the overall motion (around 0.01 on the scale used in Fig.~\ref{fig:velocity_muc}).

% For slightly larger values of the Coulomb friction coefficient values, e.g. for $\mu_c=0.10$ in Fig.~\ref{fig:velocity_muc}(b), the particle-bottom friction affects both the translational and rotational motion. The particle rotates throughout the oscillatory motion, as indicated by non-zero values of the dash-dotted curve. However, the rotational velocity is not sufficiently large to match the velocity of the bottom, which is indicated by the solid curve.
% When the bottom velocity exceeds that of the part of the particle in contact with the bottom, the particle experiences a positive acceleration due to the Coulomb friction. This force is proportional to $\mu_c$ but is independent of the velocity difference between the particle and bottom. Therefore, the slope (i.e. the acceleration) of the dash-dotted curve remains constant until the dash-dotted curve intersects the solid curve and the velocities match. After this point, the process reverses. This type of particle motion is commonly referred to as rolling motion with slip.     

% When the Coulomb coefficient is sufficiently large, e.g. when $\mu_c=0.2$ in Fig.~\ref{fig:velocity_muc}(c), the particle rolls without slip throughout the oscillatory motion, such that the dash-dotted curve overlaps the solid curve. Note that our experiments fall into this regime. 
% Increasing $\mu_c$ further does not increase the friction force or affect the particle motion. 
% Finally, it is worth noting that the amplitudes of the relative particle-fluid velocities (dotted curves) decrease as friction becomes more important. 

% \begin{figure}[ht]
%     \includegraphics[width=\linewidth]{Figures/vel_muc.png}
%     \caption{Velocities as a function of time, obtained from numerical simulations of a single spherical particle inside an oscillating box. The data is normalized by the velocity amplitude of the box and shown for three different values of the Coulomb friction coefficient $\mu_c$. The different lines indicate the velocity of the box (solid), the particle velocity in the lab frame (dashed), the particle velocity relative to the box (dotted), and the velocity of the point of the particle in contact with the bottom (dash-dotted). The simulations are carried out with $A/D=0.909$, $\delta/D\approx0.0265$, $\Gamma=0.75$, and $s=7.5$.}
%     \label{fig:velocity_muc}
% \end{figure}

% In Fig.~\ref{fig:ArA_mucGamma}, we present our numerical simulation results for $A_r/A$ as a function of $\mu_c/\Gamma$, which sets the relative importance of particle-bottom friction\citep{overveld2022numerical}. When increasing $\mu_c/\Gamma$ from 0.0 to 0.27, there is a smooth transition from $A_r/A\approx0.778$, as the particle slides over the bottom, to $A_r/A\approx0.565$, as the particle rolls without slip. At intermediate values, the particle rolls with slip. 

% For the particle to roll without slipping, the Coulomb force must always exceed the force $\boldsymbol{F}_c$ based on the inertia of the particle (see Eq.~\eqref{eq:rotationfrictionforce}). Here we have assumed that the particle rotation is solely due to particle-bottom friction. The condition for rolling without slipping is then given by
% \begin{equation}\label{eq:rollcondition}
% \begin{split}
%     \frac{\mu_c}{\Gamma} & \geq \frac{2}{5}\frac{s}{s-1}\frac{A_r}{A}, \\
%     & \gtrsim \frac{4s/5}{\sqrt{(9\delta/D)^2(2\delta/D+1)^2+(9\delta/D+14s/5+1)^2}}, \\
% \end{split}
% \end{equation}
% where we have used the solution to the BBO equation (Eq.~\eqref{eq:BBO_friction}). For the simulations discussed in this appendix, with $\delta/D\approx0.0265$, we obtain $\mu_c/\Gamma\gtrsim0.270$, which is indicated in Fig.~\ref{fig:ArA_mucGamma}. 
% The condition in Eq.~\eqref{eq:rollcondition} further confirms that the ratio $\mu_c/\Gamma$ determines the magnitude of particle-bottom friction and, consequently, the particle rotation.

% Finally, we have shaded the region in Fig.~\ref{fig:ArA_mucGamma} that encompasses all our experimental data. We have estimated that $\mu_c\approx0.3$ for the interface between glass bottom and stainless steel particles \citep{engineering_toolbox}.
% While the value of $\mu_c$ in the experiments may be slightly larger than 0.3, our results remain unchanged since it does not affect the relative particle-fluid motion. The value of $A_r/A$ remains constant above $\mu_c/\Gamma\approx0.27$.
% Nonetheless, Fig.~\ref{fig:ArA_mucGamma} emphasizes the importance of keeping $\Gamma$ (approximately) constant in our experiments. If $\Gamma$ were varied such that $\mu_c/\Gamma\lesssim0.27$, the particle motion would transition from rolling without slipping, to rolling with slip or sliding, depending on the specific value of $\mu_c/\Gamma$.

% Based on the shaded region in Fig.~\ref{fig:ArA_mucGamma}, we can conclude that in our experiments, where the relative importance of particle-bottom friction is constant, the particles always roll without slipping. As a result, keeping $\mu_c/\Gamma$ constant results in a constant value of $A_r/A$.

% \begin{figure}[ht]
%     \includegraphics[width=\linewidth]{Figures/ArA_mucGamma.png}
%     \caption{The ratio $A_r/A$ obtained from numerical simulations of a single spherical particle in an oscillating box. The three filled symbols correspond to the cases shown in Fig.~\ref{fig:velocity_muc}. Our experimental data fall within the gray area, where we have assumed that $\mu_c\approx0.3$.
%     The dotted line at $A_r/A=0.565$ indicates the constant value of $A_r/A$ for $\mu_c/\Gamma>0.27$.
%     The red and blue lines at $A_r/A\approx0.80$ and $A_r/A\approx0.58$ represent the solutions of the Basset-Boussinesq-Oseen (BBO) equation, given by Eqs.~\eqref{eq:BBO_frictionless}~and~\eqref{eq:BBO_friction}, respectively. The dashed vertical line corresponds to $\mu_c/\Gamma=0.27$ (see Eq.~\eqref{eq:rollcondition}), above which the particle rolls throughout the oscillatory motion.}
%     \label{fig:ArA_mucGamma}
% \end{figure}
